# Supplementary material for: Crystal field, ligand field, and interorbital effects in two-dimensional transition metal dichalcogenides across the periodic table
Source: arXiv:1810.01302 ancillary file (2018-10-02)
Supplement: Supplementary file 1 [file suppl.pdf]

# Supplemental Material for
# "Crystal field, ligand field, and interorbital effects in two-dimensional transition metal dichalcogenides across the periodic table"

Diego Pasquier and Oleg V. Yazyev
*Institute of Physics, Ecole Polytechnique Fédérale de Lausanne (EPFL), CH-1015 Lausanne, Switzerland*

## I. HIGHER-ENERGY BANDS OF 1*T*-TAS$_2$

In the main text, we have discussed the effect of including explicitly high-energy states (i.e. tantalum 6$s$ and 6$p$ states, and sulfur 3$d$ states) in the construction of the Wannier functions, without showing the corresponding band structures. In Fig. 1, we show the DFT bands including several excited-states bands above the two $e_g$ bands. We see that the bands are highly entangled, so that one cannot simply take a set of isolated bands for wannierization. Fig. 1 also shows the bands in the 27-band *spddsp* model, with the orbital weight of the five $d$ Wannier functions as a color code. The $d$-like Wannier functions contribute mainly to the five bands close to the Fermi level, which we have referred to as the $d$ bands in the main text. However, it is clear that the $d$ Wannier functions also contribute to the lower-energy and higher-energy bands (especially to the bottom of the $p$ bands), indicating the formation of bonding and antibonding states with the corresponding Wannier functions. In Fig. 1, we show, with dashed red lines, the bands obtained with the 13-band *spd* model. These bands match exactly the DFT bands, except at the top of the $e_g$ bands, because there is a small overlap with the higher-energy bands.

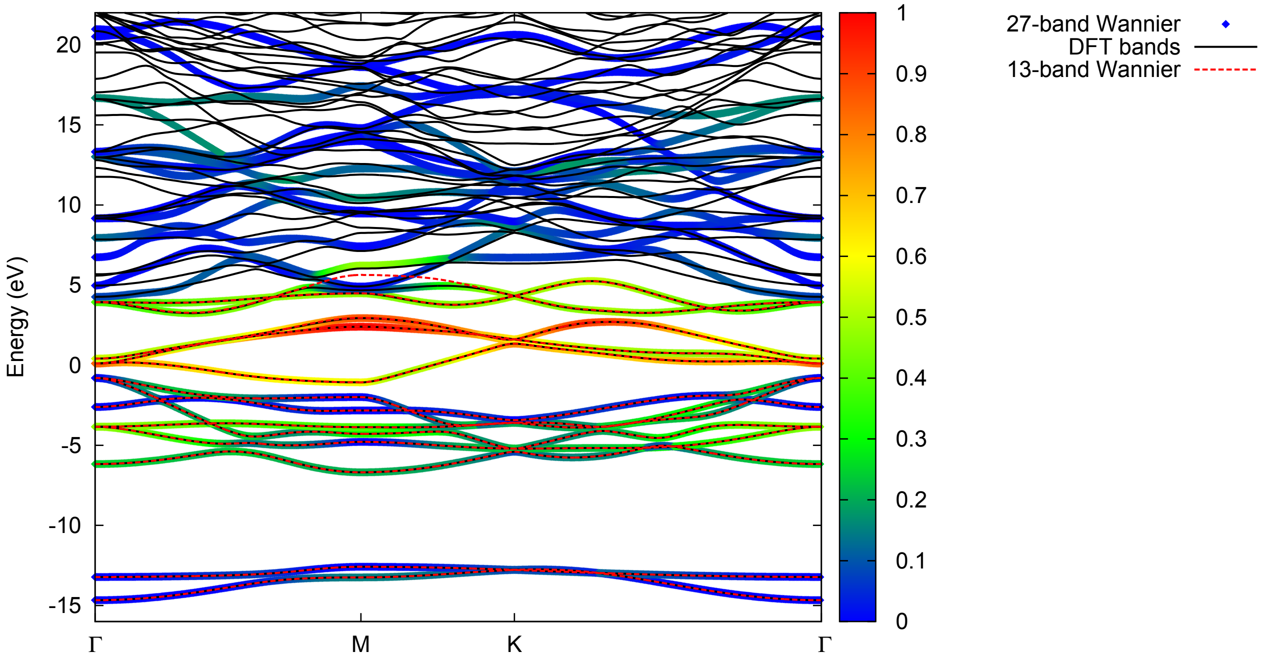


FIG. 1. Bands for the 27-band *spddsp* model of monolayer 1*T*-TaS$_2$ with the orbital weight of the $d$ Wannier functions as a color code. The Fermi level is set to zero. The DFT bands, including the high-energy bands, are shown with continuous black lines. The dashed red lines correspond to the bands of the 13-band *spd* model.

## II. BAND STRUCTURES OF THE CONSIDERED MATERIALS

In the main text, we have not shown the band structures for all the materials considered. Here, we present the missing band structures, for the 13-band and 5-band models, for both the $1T$ and $1H$ phases. Note that the DFT bands are not explicitly shown, but they match the bands of the 13-bands models up to some minor differences.

### A. $4d$ disulfides trend

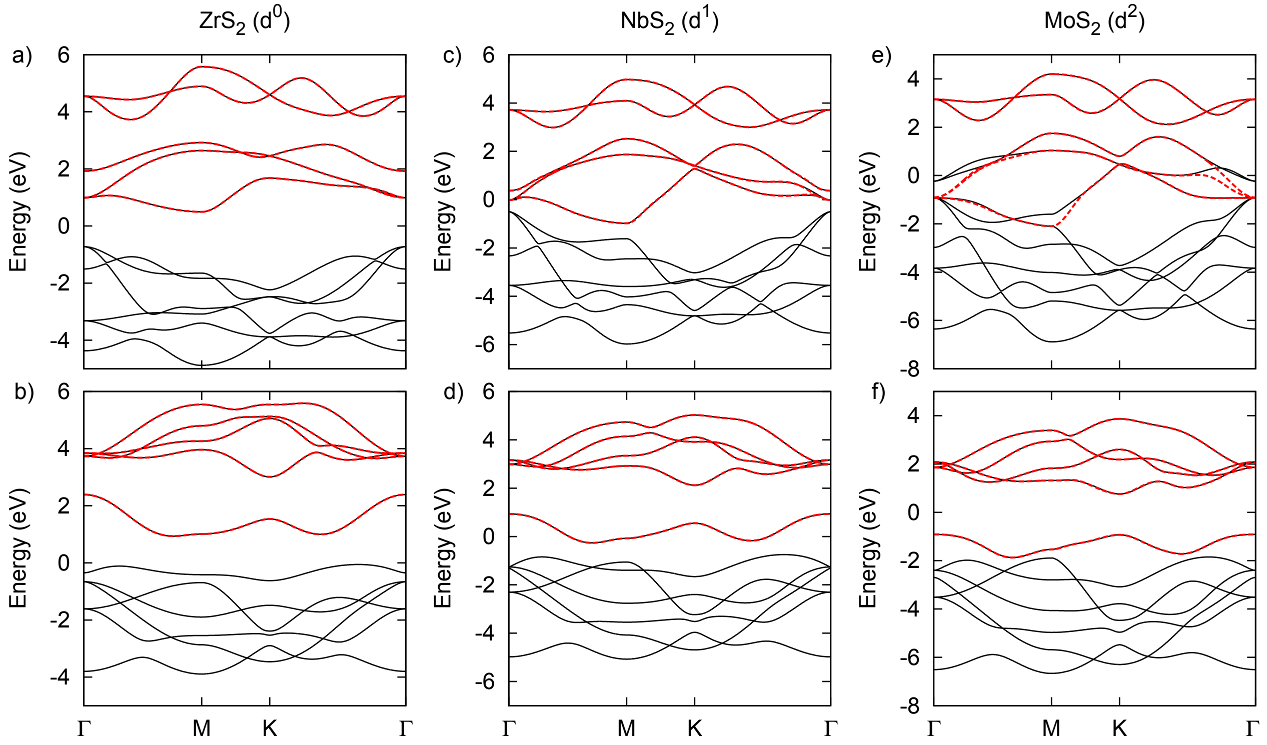


FIG. 2. Band structure calculated from first principles for monolayers of (a) $1T$-$ZrS_2$, (b) $1H$-$ZrS_2$, (c) $1T$-$NbS_2$, (d) $1H$-$NbS_2$, (e) $1T$-$MoS_2$ and (f) $1H$-$MoS_2$. The Fermi level is set to zero. Continuous black lines correspond to the 13-band *spd* model and red dashed lines correspond to the 5-band $d$ model.

In Figs. 2 and 3, the calculated band structure for the $4d$ transition metal disulfides trends are shown. As for the $5d$ disulfides cases, the $p$-like and $d$-like bands are well separated in energy in the $d^0$-$d^2$ range. At $n \leq 3$ $d$ electrons, the $p$ and $d$ bands overlap in energy, so that disentanglement is necessary to construct the 5-band models.

### B. $PdS_2$

Fig. 4 shows the calculated PBE band structures of monolayer $PdS_2$ in the $1T$ and $1H$ phases. As we have stated in the main text, the relaxed atomic structure of $PdS_2$ in the $1H$ polymorph is characterized by a significant shortening of the S-S distance, leading to a band structure qualitatively different from the other considered materials. On the other hand, the calculated band structure of $1T$-$PdS_2$ is similar to that of other late-group $1T$ TMDs.

### C. $5d$ disulfides trend

In Fig. 5, we show the band structures for the $5d$ disulfides trend that are not presented in the main text ($WS_2$, $OsS_2$ and $IrS_2$).

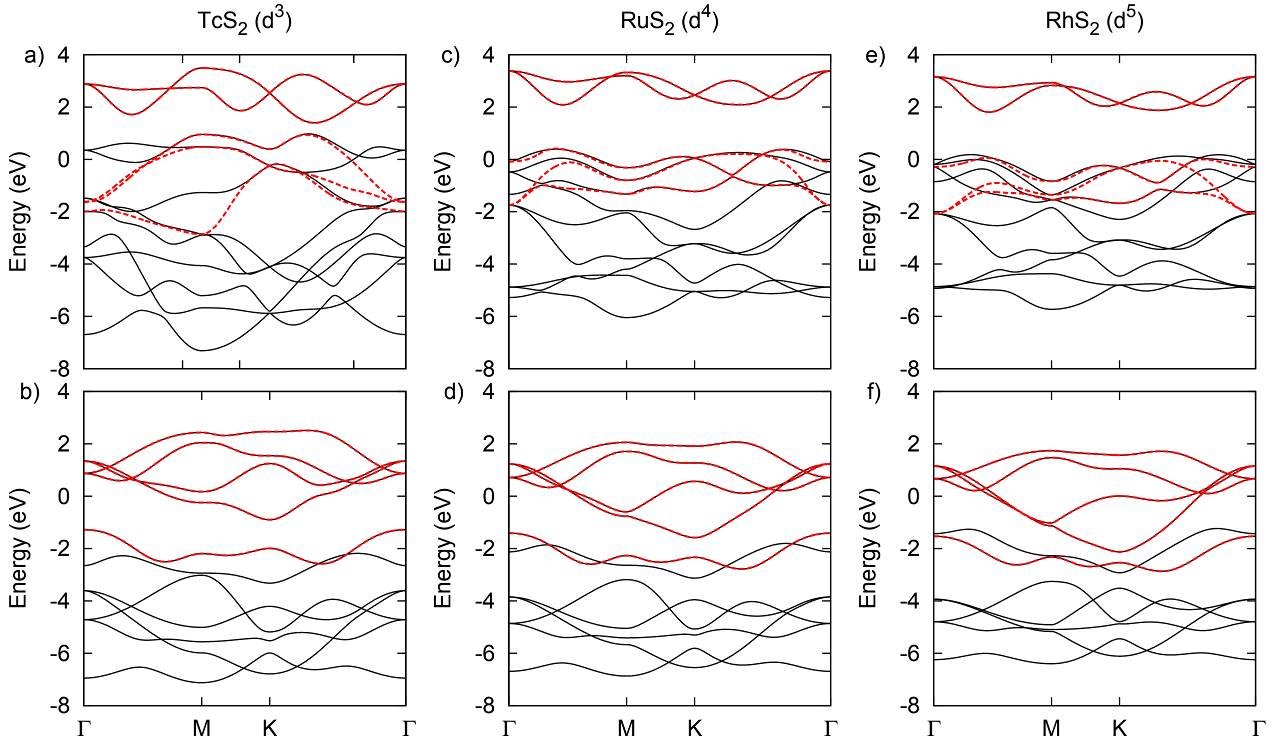


FIG. 3. Band structures calculated from first principles for monolayers of (a) 1$T$-$TcS_2$, (b) 1$H$-$TcS_2$, (c) 1$T$-$RuS_2$, (d) 1$H$-$RuS_2$, (e) 1$T$-$RhS_2$ and (f) 1$H$-$RhS_2$. The Fermi level is set to zero. Continuous black lines correspond to the 13-band *spd* model and red dashed lines correspond to the 5-band $d$ model.

### D. $d^1$ disulfides trend

In Fig. 6, we present the calculated band structures for the $nd^1$ trend. In the case of 1$T$-$VS_2$, there is some entanglement between the $t_{2g}$ and $p$ bands (i.e. band inversion at the Γ point), explaining why the bands in the 13-band and 5-band models do not match exactly.

### E. $TaX_2$

In Fig. 7, band structures for the $TaX_2$ trend are shown. The $p$ and $d$ bands are well separated for $TaS_2$ and $TaSe_2$, but overlap in energy for $TaTe_2$.

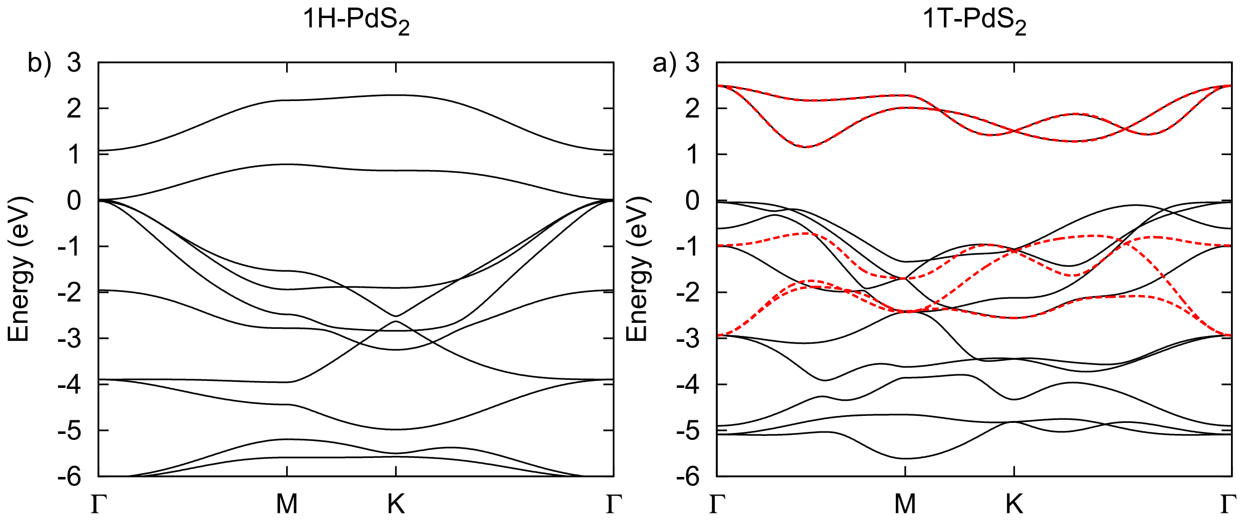


FIG. 4. Band structure calculated from first principles for monolayers of (a) $1T$-$PdS_2$. The Fermi level is set to zero. Continuous black lines correspond to the 13-band *spd* model and red dashed lines correspond to the 5-band *d* model. (b) Calculated band structure for $1H$-$PdS_2$.

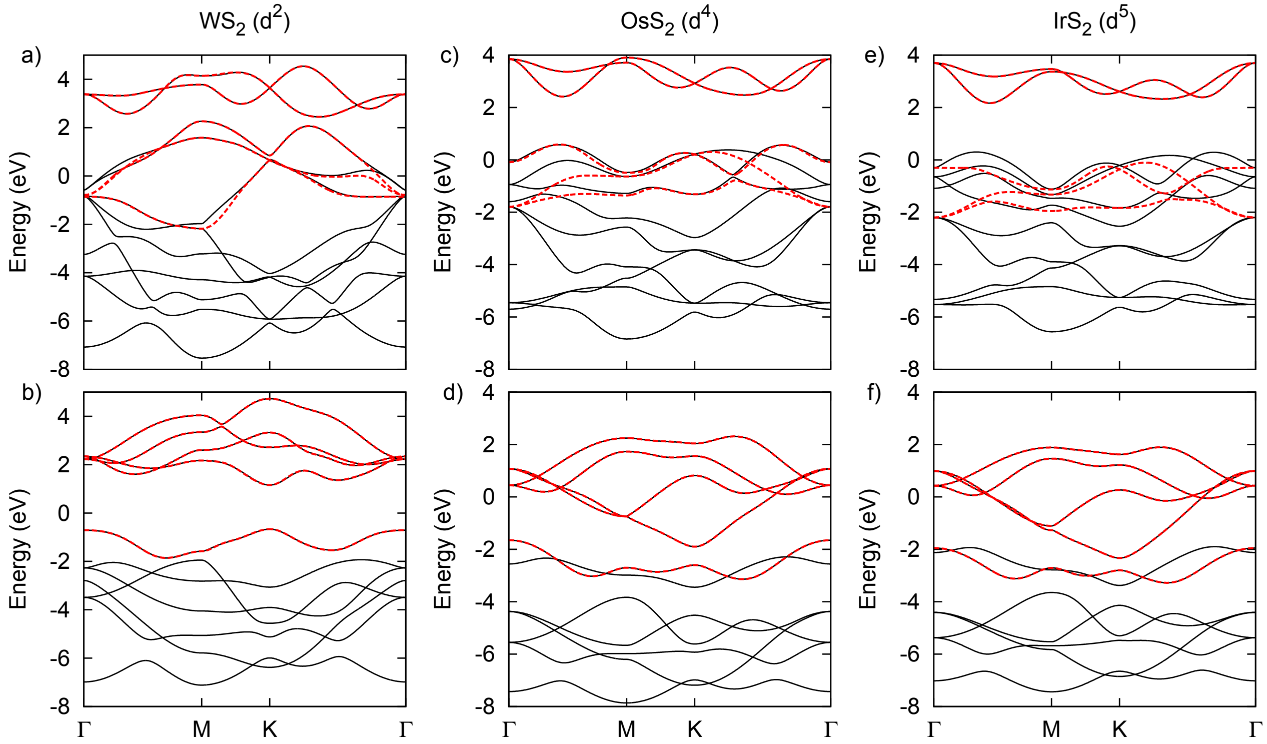


FIG. 5. Band structure calculated from first principles for monolyers of (a) $1T$-$WS_2$, (b) $1H$-$WS_2$, (c) $1T$-$OsS_2$, (d) $1H$-$OsS_2$, (e) $1T$-$IrS_2$ and (f) $1H$-$IrS_2$. The Fermi level is set to zero. Continuous black lines correspond to the 13-band *spd* model and red dashed lines correspond to the 5-band *d* model.

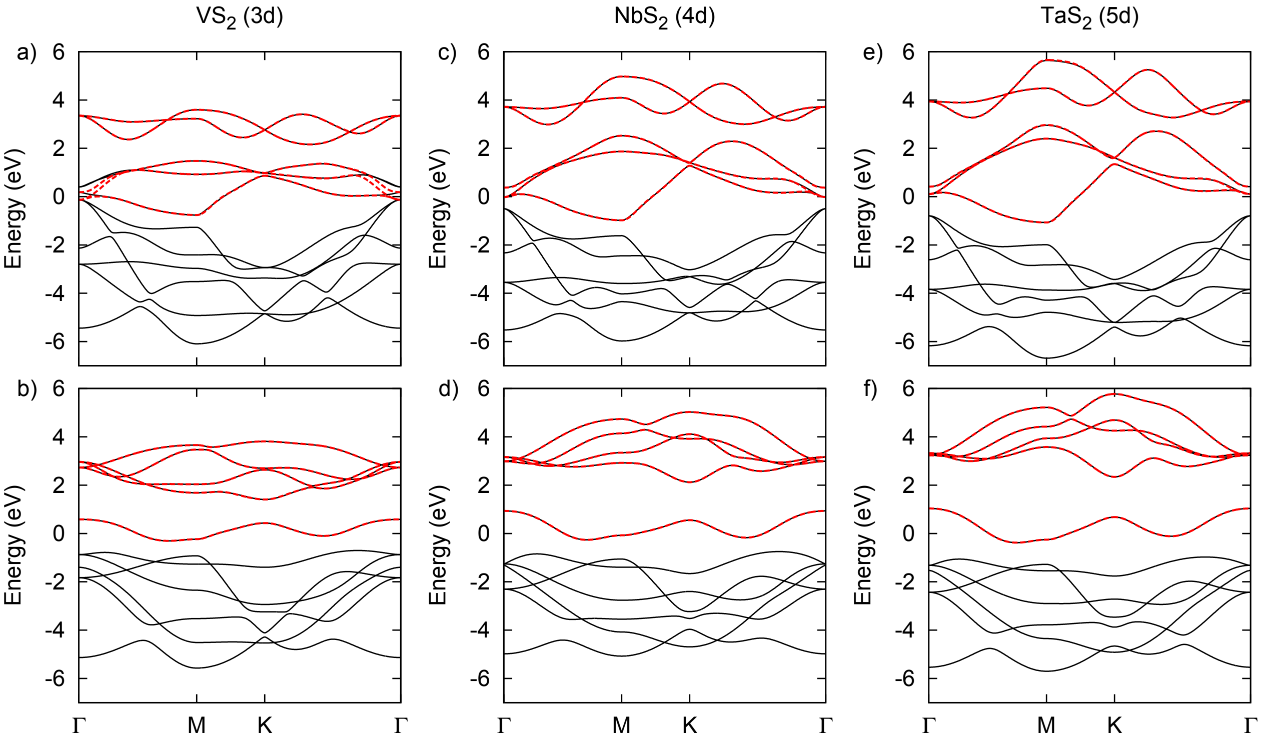


FIG. 6. Band structure calculated from first principles for monolayers of (a) $1T$-$VS_2$, (b) $1H$-$VS_2$, (c) $1T$-$NbS_2$, (d) $1H$-$NbS_2$, (e) $1T$-$TaS_2$ and (f) $1H$-$TaS_2$. The Fermi level is set to zero. Continuous black lines correspond to the 13-band *spd* model and red dashed lines correspond to the 5-band $d$ model.

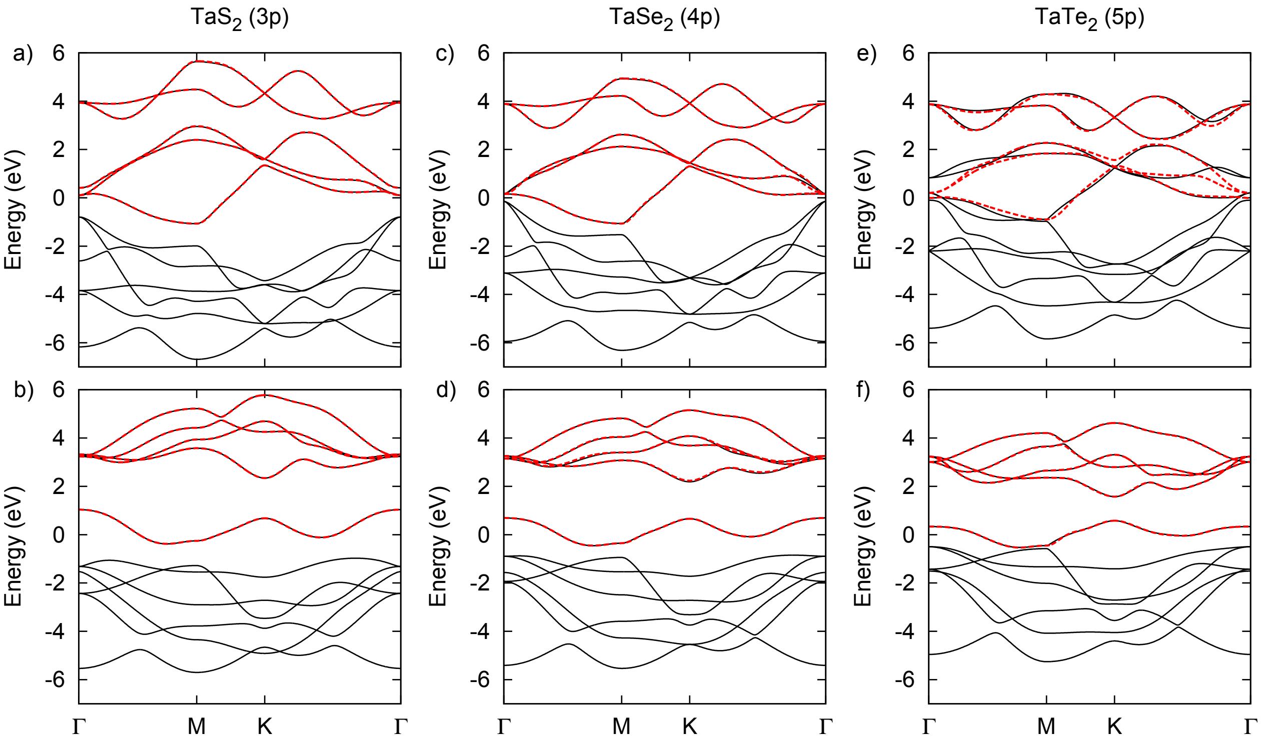


FIG. 7. Band structure calculated from first principles for monolayers of (a) $1T$-$TaS_2$, (b) $1H$-$TaS_2$, (c) $1T$-$TaSe_2$, (d) $1H$-$TaSe_2$, (e) $1T$-$TaTe_2$ and (f) $1H$-$TaTe_2$. The Fermi level is set to zero. Continuous black lines correspond to the 13-band *spd* model and red dashed lines correspond to the 5-band $d$ model.
